# Supplementary material for: Uncertainty-Aware Semantic Augmentation for Neural Machine Translation
Source: arXiv:2010.04411 source file (2020-10-09)
Supplement: Supplementary file 1 [file appendix.tex]

\section{Study of Different $N$}
\label{sec:supplemental-N}
To determine the number of synthetic source sentences $N$ in our system beforehand, we conduct experiments on Chinese-English and English-German translation tasks to test how it affects the translation performance. We vary the value of $N$ from 1 to 9 with 2 as step size and the results are reported on validation sets (Table~\ref{table-N}). We can find that the
translation performance achieves substantial improvement with $N$ increasing from 1 to 3. However, with $N$ set larger than 3, we get little improvement. To make a trade-off between the translation performance and the computation complexity, we set $N$ as 3 in our experiments.

\begin{table}[ht!]
	\begin{center}
	%\footnotesize
		\begin{tabular}{l|p{1.5cm}<{\centering}p{1.5cm}<{\centering}p{1.5cm}<{\centering}}
		%\begin{tabular}{l|ccc}
			\hline
			\multirow{2}{*}{$N$} & NIST & WMT'18 & WMT'16\\
			~ & Zh-En & Zh-En & En-De\\
			\hline
			\hline
			1 & 43.09 & 23.01 & 24.50\\
			3 & 44.01 & 23.80 & 25.22\\
			5 & 43.92 & 23.89 & 25.30\\
			7 & 44.09 & 23.77 & 25.31\\
			9 & 44.14 & 23.68 & 25.37\\
			\hline
		\end{tabular}
	\end{center}
	\caption{\label{table-N}The experiments on the number of synthetic source sentences over Chinese-English and English-German validation sets.}
\end{table}

\begin{table}[t!]
	\begin{center}
	%\footnotesize
		%\begin{tabular}{l|p{0.8cm}<{\centering}|p{1.5cm}<{\centering}p{1.5cm}<{\centering}}
		\begin{tabular}{l|p{1.0cm}<{\centering}|p{1.7cm}<{\centering}p{1.7cm}<{\centering}}
		    %\hline
			\hline
			\multirow{4}{*}{$\hbar$} & \multirow{4}{*}{BLEU} & \multicolumn{2} {c} {Edit Distance}\\
			\cline{3-4}
			~ & ~ & SYN & SYN\\
			~ & ~ & vs. & vs. \\
			~ & ~ & REAL & SYN \\
			%\multirow{2}{*}{${\rm h}_{bias}$} & \multirow{2}{*}{BLEU} & \multicolumn{2} {c} {Edit Distance}\\
			%\cline{3-4}
			%~ & ~ & SYN vs. REAL & SYN vs. SYN\\
			\hline
			\hline
		    \multicolumn{4} {c} {LDC Chinese-English} \\
		    \hline
		    BS-3 & 20.87 & 8.70 & 5.14 \\
		    \hline
			0.0 & 10.71 & 17.26 & 19.18 \\
			1.0 & 11.99 & 17.17 & 18.91 \\
			2.5 & 17.60 & 12.80 & 12.38 \\
			4.5 & 19.47 & 9.93 & 6.24 \\
			7.0 & 20.30 & 9.07 & 4.35 \\
			\hline
			\hline
		    \multicolumn{4} {c} {WMT'18 Chinese-English} \\
			\hline
			%\multirow{2}{*}{${\rm h}_{bias}$} & \multicolumn{2} {c|} {BLEU} & \multicolumn{2} {c} {ED}\\
			%\cline{2-5}
			%~ & CS-3 & BS-3 & SYN vs. REAL & SYN vs. SYN\\
			%\hline
			%\hline
			BS-3 & 34.47 & 10.74 & 4.73\\
		    \hline
			0.0 & 24.01 & 22.55 & 21.41 \\
			1.0 & 25.22 & 22.03 & 21.09\\
			2.5 & 31.29 & 12.58 & 12.24 \\
			4.5 & 32.96 & 9.31 & 6.29 \\
			7.0 & 33.81 & 9.37 & 5.24 \\
			\hline
			\hline
		    \multicolumn{4} {c} {WMT'16 English-German} \\
			\hline
			%\multirow{2}{*}{${\rm h}_{bias}$} & \multicolumn{2} {c|} {BLEU} & \multicolumn{2} {c} {ED}\\
			%\cline{2-5}
			%~ & CS-3 & BS-3 & SYN vs. REAL & SYN vs. SYN\\
			%\hline
			%\hline
			BS-3 & 30.11 & 9.59 & 4.36 \\
		    \hline
			0.0 & 19.84 & 15.60 & 15.75 \\
			1.0 & 20.57 & 15.22 & 15.26 \\
			2.5 & 26.44 & 10.45 & 10.23 \\
			4.5 & 28.07 & 8.38 & 3.95 \\
			7.0 & 29.25 & 7.29 & 2.71 \\
			\hline
		\end{tabular}
	\end{center}
	\caption{\label{table-h-bias}The BLEU scores and the edit distances of synthetic source sentences based on 3 synthetic sentences and real source sentences. ``BS-3'' indicates that the 3 synthetic sentences are generated by beam search with a beam size of 3.}
\end{table}
\section{Study of Different $\hbar$}
\label{sec:supplemental-h-bias}
The introduction of the hyperparameter $\hbar$ aims at acquiring the proper quantity of uncertainties. To investigate the effect of it, we quantify: (1) the diversity using the edit distance among the synthetic source sentences and (2) the quality using BLEU scores
of synthetic source sentences, with respect to various values of $\hbar$. 

For each target sentence in validation sets, we generate $N=3$  synthetic source sentences using our controlled sampling strategy. Table~\ref{table-h-bias} shows the results. The BLEU scores were computed regarding the multiple synthetic sentences as a document. As in (Imamura et al., 2018), the edit distances are computed for two cases: (1) SYN vs. REAL, the average distance between a synthetic source sentence (SYN) and the real source sentence (REAL). Note that this value also indicates translation quality because it is a source for computing the word error rate (smaller value represents better quality). (2) SYN vs. SYN, the average distance among synthetic source sentences of a target sentence (${\rm C}_{3}^{2}=3$ combinations per target sentence). We can find that when $\hbar$ tends to 0 our controlled sampling method achieves lowest BLEU scores but highest edit distances. However, if we increase $\hbar$ gradually, it can be quickly simplified to greedy search. Among all values of $\hbar$ in Table~\ref{table-h-bias}, $\hbar=2.5$ is a proper setting as it demonstrates relatively higher BLEU scores and lower word error rates (SYN vs. REAL) as well as more of diversity (SYN vs. SYN) in corpora. Therefore, we set $\hbar$ as 2.5 in all of our experiments.

\section{Learning Curves of Loss Functions.}
Figure~\ref{fig:loss} shows the learning curves of three loss items, in which ``MLE-loss'' indicates the combination of $\ell_{\rm mle}({\rm \bf x}, {\rm \bf y})$ and $\ell_{\rm mle}(\mathbf{\bar{\rm \bf x}}, {\rm \bf y})$ while ``SCN-loss'' represents  $\ell_{\rm sem}$. We find that ``MLE-loss'' drops rapidly within the first few steps and then presents the state of oscillation. It is common that introducing synthetic data into semantic constrained training can make the loss curves not very smoothing. In addition, the behavior of ``SCN-loss'' demonstrates a pattern that we observed often: $\rm KL$ (Eq. (\ref{eq:loss-scn})) spikes early in training while the model can encode information in ${\rm \bf z}$ (or $\mathbf{\bar{z}}$) cheaply, then drops substantially once it begins paying the full $\rm KL$-divergence penalty ($\gamma=1.0$), and keeps dropping gradually.

\begin{figure}[t!]
	\centering
	\includegraphics[width=0.5\textwidth]{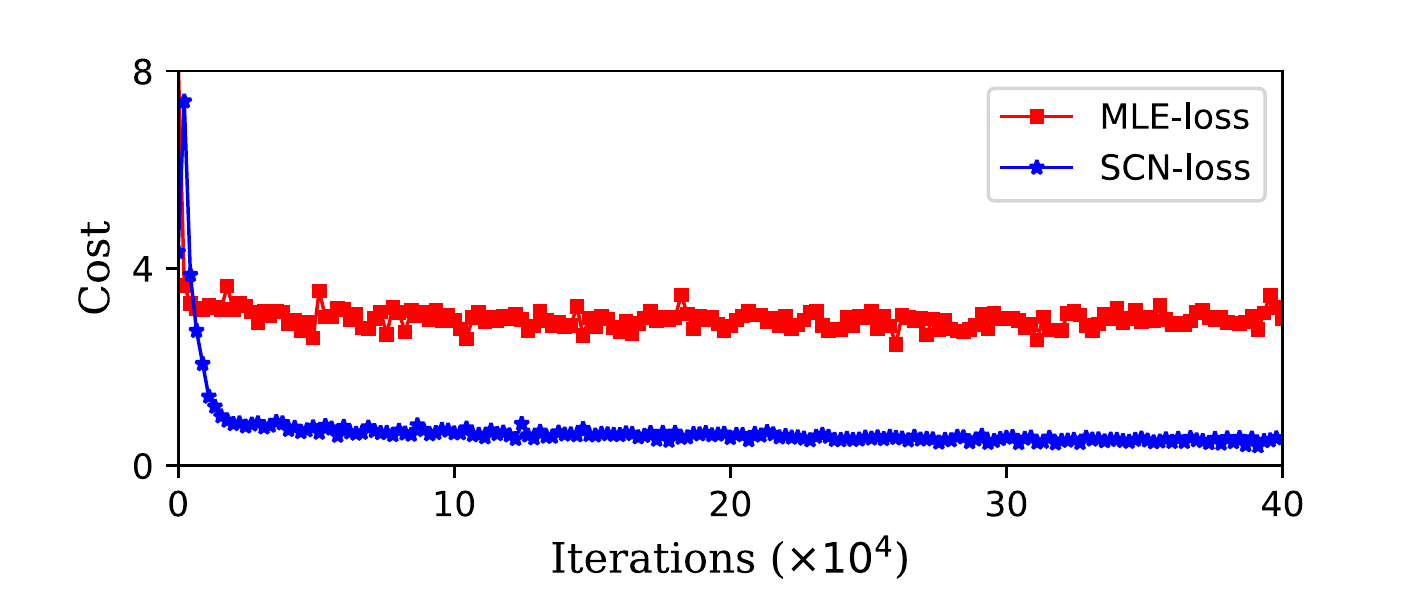}
	\caption{\label{fig:loss}Learning curves of loss functions.}
\end{figure}

\begin{table}[t!]
	\begin{center}
	%\footnotesize
		\begin{tabular}{l|c|c}
			\hline
			Model & Method & BLEU\\
			\hline
			\hline
			\multirow{3}{*}{U-SemAug} & BS-3 & 23.41\\
			~& MS-3 & 23.74\\
			~& CS-3 & 24.10\\
			\hline
		\end{tabular}
	\end{center}
	\caption{\label{bleu-table-cs}Effect of different methods to generate multiple synthetic data. ``BS'', ``MS'' and ``CS'' denote the beam search, multinomial sampling and our controlled sampling methods, respectively. ``-3'' indicates we synthesize 3 source sentences for each target sentence.}
\end{table}

\section{Effect of Controlled Sampling}
In Table~\ref{table-controlled-sampling}, the widely used multinomial sampling (MS) and beam (greedy) search (BS) can be viewed as two special cases of our introduced controlled sampling (CS). As shown in Table~\ref{bleu-table-cs}, our controlled sampling method achieves the best result among them on the validation set. We think that reasonable uncertainties can be mined via our controllable sampling strategy.

\section{Case Study}
Table~\ref{tb:examples} shows the comparison of translation results of Transformer and U-SemAug for several translation examples. In the first case, the results of the Transformer suffer from adequacy and accuracy: 1) translates ``\begin{CJK*}{UTF8}{gbsn}徽文化非遗传承\end{CJK*}'' into ``Hui culture'', where ``\begin{CJK*}{UTF8}{gbsn}非遗\end{CJK*}'' and ``\begin{CJK*}{UTF8}{gbsn}传承\end{CJK*}'' are mistakenly untranslated; 2) ``\begin{CJK*}{UTF8}{gbsn}非遗\end{CJK*}'' is literally translated into ``non-genetic'' without considering its real meaning, which is also exposed an under-estimation problem of rare words. In contrast, U-SemAug handles this case almost well. For the second and third cases, the generated sentences of U-SemAug are reasonable and acceptable to the Transformer. In the last case, our model retains a very important word ``travel'', which are missing in the Transformer results.

\begin{table*}[t!]
	%\footnotesize
	\centering
	\begin{tabular}{c|p{13cm}}
		\toprule[1.25pt]
		\multicolumn{2} {c} {\bf Case 1} \\
		\toprule[1.25pt]
		Source & \begin{CJK*}{UTF8}{gbsn}
			由于徽文化非遗传承主要依赖口传面授，许多非遗濒临失传，运用数字化技术保存和保护势在必行 。
		\end{CJK*}\\
		\hline
		Reference & As the inheritance of intangible cultural heritage projects of Anhui province mainly relies on oral and face-to-ace passage, many intangible cultural heritage projects are on the verge of failing to be handed down from past generations. So the application of digital technology for conservation is imperative.\\
		\hline
		Transformer & As \textcolor{blue}{Hui culture} mainly relies on oral and face-to-face \textcolor{blue}{transmission} for \textcolor{blue}{non-genetic} inheritance, many \textcolor{blue}{non-genetic heritage} is on the verge of extinction, and it is imperative to preserve and protect it by digital technology.\\
		\hline
		U-SemAug & Because \textcolor{red}{the inheritance of Hui culture intangible cultural heritage} mainly depends on oral and face-to-face \textcolor{red}{teaching}, many \textcolor{red}{intangible cultural heritage} are on the verge of \textcolor{blue}{losing transmission}, so it is imperative to preserve and protect it by digital technology.\\
		\bottomrule[1.25pt]
		\multicolumn{2} {c} {\bf Case 2} \\
		\toprule[1.25pt]
		Source & \begin{CJK*}{UTF8}{gbsn}
			我认为我们可以重新启动这些品牌，而且现在时间正合适。
		\end{CJK*}\\
		\hline
		Reference & We can bring those brands back up again, so I think the time is right.\\
		Transformer & I think we can \textcolor{blue}{restart} these brands, and the time is right.\\
		\hline
		U-SemAug & I think we can \textcolor{red}{relaunch} these brands, and now is the right time.\\
		\bottomrule[1.25pt]
		\multicolumn{2} {c} {\bf Case 3} \\
		\toprule[1.25pt]
		Source & \begin{CJK*}{UTF8}{gbsn}
			根据通航需要，老万福河航道采取养护改造的方式，对局部水深进行了浚深，局部急弯进行裁弯取直等，通航条件得以改善。
		\end{CJK*}\\
		\hline
		Reference & According to the navigation needs, the old Wanfu River channel takes the mode of conservation and transformation. Dredging was conducted on the local depth and curve cut-off on the local sharp bend. Then the navigation conditions can be improved.\\
		\hline
		Transformer & According to the needs of navigation, the old Wanfu River waterway is maintained and renovated, with deepened water \textcolor{blue}{depth in some parts and straight bends in some sharp bends}, thus improving navigation conditions.\\
		\hline
		U-SemAug & According to the navigation needs, the old Wanfu river channel adopts the way of maintenance and reconstruction. \textcolor{red}{The local water depth is dredged, the local sharp bend is cut and straightened.} Thus the navigation conditions are improved.\\
		\bottomrule[1.25pt]
		\multicolumn{2} {c} {\bf Case 4} \\
		\toprule[1.25pt]
		Source & \begin{CJK*}{UTF8}{gbsn}
			俄中两国警察部门合作将提升本国公民到对方国家旅游的安全感。
		\end{CJK*}\\
		\hline
		Reference & The cooperation between the Russian and Chinese police departments will enhance the security sense of their citizens to each other's national tourism.\\
		\hline
		Transformer & The cooperation between the police departments of Russia and China will enhance the sense of security for their citizens \textcolor{blue}{to each other's countries.}\\
		\hline
		U-SemAug & The cooperation between the police departments of Russia and China will enhance the sense of security of their citizens \textcolor{red}{to travel to each other's countries.}\\
		\bottomrule[1.25pt]
	\end{tabular}
	\caption{\label{tb:examples}Comparison of translation results of Transformer and our U-SemAug for several cases on WMT18 Zh$\rightarrow$En task. \textcolor{red}{Red} parts represent correct translations while \textcolor{blue}{blue} ones indicate incorrect translations.}%, where \#1 is the original input and both \#2 and \#3 are its semantically-equivalent counterparts.
\end{table*}
